# Supplementary material for: Parton-shower effects in polarized deep inelastic scattering
Source: arXiv:2404.07702 source file (2024-07-23)
Supplement: Supplementary file 1 [file appendix.tex]

\section{Appendix}
\label{app}

use appendix only if relevant
